# Supplementary material for: EMNS /Imz/ Corpus: An emotive single-speaker dataset for narrative storytelling in games, television and graphic novels
Source: arXiv:2305.13137 source file (2023-05-25)
Supplement: Supplementary file 1 [file appendix.tex]

\newpage
\appendix

\section{Experiments} \label{appendix: experiments}
% Did those who were happier identify emotion better?
% Does adding reverb improve the genuine score?

% NOTES:
% Disgust/Angry are confused on the low and high expression levels. happy/neutral are confused with each other on low expressiveness levels when the actor self repoted low expresiveness.
% Sarcastic can be confused with other emotions in the low expressive levels because it is very context-dependent.
% Adding environmental noise further improved the believably of acted recording

\subsection{Dataset comparison}
To evaluate the effectiveness of the Emotive Narrative Storytelling (EMNS) dataset, a survey was conducted with 19 native and non-native English speakers. The survey aimed to compare the EMNS dataset with four comparable datasets, namely Crema-D \cite{dataset:CREMA-D}, ESD \cite{dataset:ESD}, RAVDESS \cite{dataset:RAVDESS}, and MSP-IMPROV \cite{dataset:MSP-IMPROV}.

To quantify the subjective task of emotional speech, Mean Opinion Score (MOS) was utilised. MOS commonly measures subjective tasks such as audio and video quality, speech intelligibility, and user experience. It uses a scale-based evaluation to quantify a user's perceived task quality.

In the context of the EMNS dataset, MOS was used to assess its ability to convey emotions accurately through speech. Participants were asked to rate randomly selected samples based on their ability to accurately depict the shared emotions of sadness, neutral, happy, and angry, across all five datasets. The ratings were based on three categories: the sample that best conveyed the shared emotion, the most expressive sample, and the most genuine sample.

The results showed that the EMNS dataset outperformed the other datasets in accurately conveying emotions, with 41\% of participants choosing it as the best conveying dataset. MSP-IMPROV came in second with 30\% of the votes. Regarding best conveying per emotion, EMNS outperformed all comparable datasets in \textit{sadness}, \textit{neutral}, and \textit{anger}, but underperformed in \textit{happy} due to the random selection of a low expressiveness of 2. MSP-IMPROV scored 11\% less on average, and EMNS outperformed RAVDESS by 24\%.

\begin{figure}[t]
  \centering
  \includegraphics[width=\linewidth]{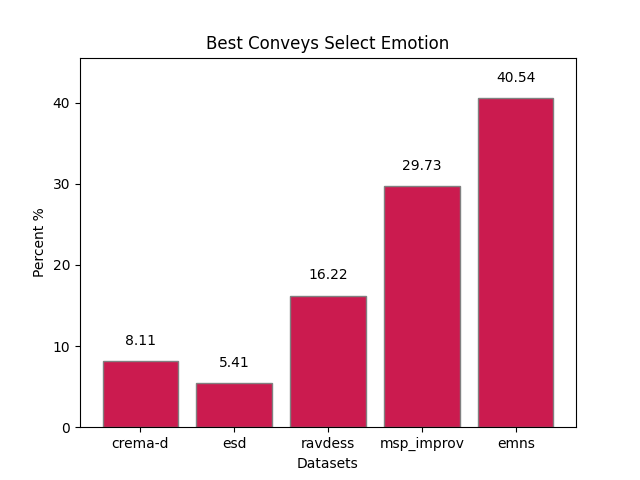}
  \caption{The Mean Opinion Score for the most effectively conveyed emotions across the five datasets and four emotions (sadness, neutral, happy, anger).}
  \label{fig:surveyed-emotion-comparison}
\end{figure}

In terms of expressiveness, the results showed that EMNS outperformed all other datasets, with 46\% of participants reporting it as the most expressive, followed by MSP-IMPROV at 29\%. The results for genuineness, however, showed room for improvement, with 38\% of participants choosing Crema-D, followed by MSP-IMPROV at 24\% and EMNS at 22\%. The full results can be seen in Table \ref{fig:surveyed-genuine-comparison}

\begin{figure}[t]
  \centering
  \includegraphics[width=\linewidth]{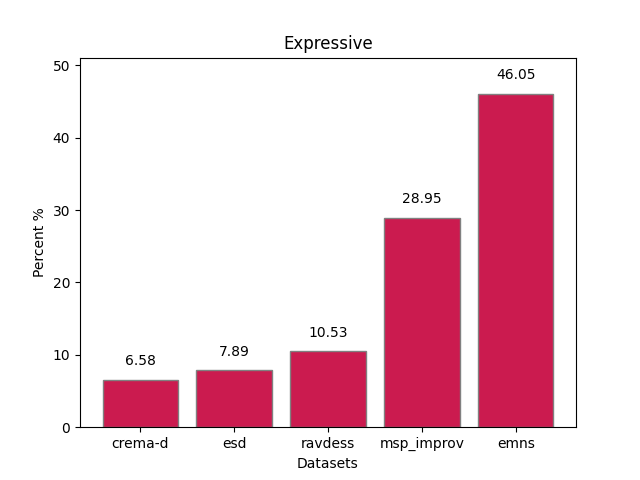}
  \caption{Perceived expressiveness comparing five datasets and four emotions (sadness, neutral, happy, anger).}
  \label{fig:surveyed-expressive-comparison}
\end{figure}

\begin{figure}[t]
  \centering
  \includegraphics[width=\linewidth]{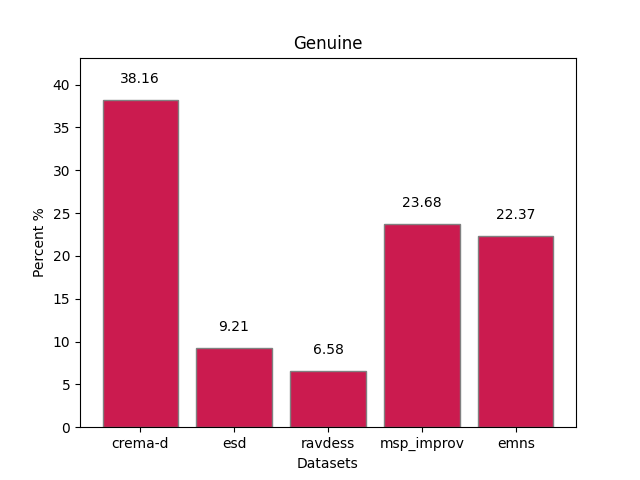}
  \caption{Perceived genuineness level across five datasets and four emotions (sadness, neutral, happy, anger). }
  \label{fig:surveyed-genuine-comparison}
\end{figure}

\subsection{Speech Synthesis}

A modified FastSpeech2 model was trained to further investigate and evaluate the effectiveness of the Emotive Narrative Storytelling (EMNS) dataset. FastSpeech2 is a state-of-the-art neural text-to-speech system that produces high-quality real-time speech output. The model features a non-autoregressive transformer architecture, allowing for fast speech generation. A critical component of FastSpeech2 is the variance adaptor. This neural network module adjusts the variance of the generated mel-spectrogram frames to match the ground-truth frames and simultaneously predicts the target frames for a given input text.

The variance adaptor can be utilised to control the emotional expressiveness of the synthesised speech. By adjusting the variance of the mel-spectrogram frames, the model can be trained to generate speech with a specific emotional tone or replicate the emotional characteristics of a particular speaker. We employed this capability to evaluate the effectiveness of the EMNS Corpus.

\begin{figure}[t]
  \centering
  \includegraphics[width=\linewidth]{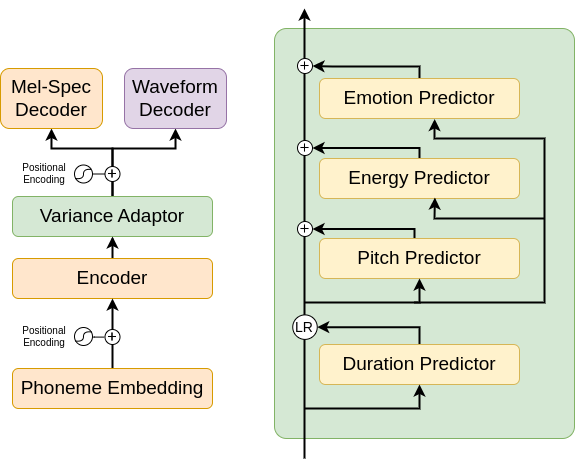}
  \caption{Modified FastSpeech 2 \cite{paper:fastspeech_2021}, with Emotion variance adaptor. Where LR is length regulators from FastSpeech}
  \label{fig:FS20-EMNS}
\end{figure}

Figure \ref{fig:FS20-EMNS} outlines the addition of an emotion predictor used to learn and synthesise emotional speech. In addition, we make modifications to the proposed loss of FastSpeech 2.

\begin{equation*}
	L = L_{mel} + \lambda L_{dur} + \alpha L_{eng} + \beta L_{pit} + \gamma L_{emo}
\end{equation*}

Where $L$ is the total loss, $L_{mel}$, $L_{dur}$, $L_{eng}$ and $L_{pit}$ are MSE loss. $\lambda$, $\alpha$, $\beta$ and $\gamma$ are hyperparameters used to control the weighting of these losses. $L_{emo}$ is a cross-entropy loss used to optimise the emotion predictor.

\subsubsection{Results}
To evaluate the quality of the synthesised speech produced by our adapted FastSpeech2 model, we trained it on the emotion datasets outlined in section \ref{sec:experiments}. The audio samples generated by the model can be accessed at \textbf{Github Link to the Audio Samples}. Subsequently, we conducted a Mean Opinion Score (MOS) survey with \textbf{NUMBER} participants to obtain a comprehensive and representative evaluation of the synthesised speech's quality.

The survey was designed to assess the efficacy of the EMNS corpus in producing emotionally expressive and non-emotionally expressive speech. It consisted of three primary components. Initially, participants were required to identify the emotions conveyed in each synthesised speech sample to evaluate the model's ability to produce speech that accurately conveyed the intended emotional tone. Secondly, the participants assessed the speech samples' genuineness based on predetermined criteria, aiming to assess how closely the synthesised speech resembled natural human speech. Finally, the participants compared the synthesised speech samples with the ground truth samples to evaluate the overall quality of the speech generated by our model.

The survey's results provide significant insights into the effectiveness of our approach and demonstrate the value of generating emotionally expressive speech. These findings will be presented in the subsequent section.

\paragraph{MOS}

\subsection{Corpus creation} \label{appendix:corpus_creation}

\begin{figure}[t]
  \centering
  \includegraphics[width=\linewidth]{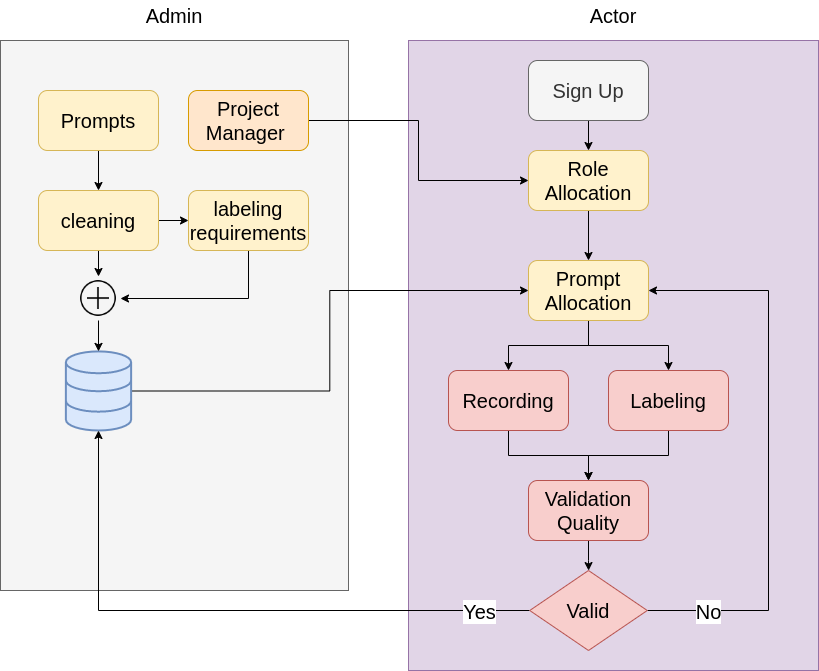}
  \caption{}
  \label{fig:FS20-EMNS}
\end{figure}
